# Supplementary material for: Correlated Spin-Flip Tunneling in a Fermi Lattice Gas
Source: arXiv:1711.02061 ancillary file (2017-11-06)
Supplement: Supplementary file 1 [file SM5.pdf]

# Supplementary Material for “Correlated Spin-Flip Tunneling in a Fermi Lattice Gas”

Wenchao Xu,<sup>1</sup> William Morong,<sup>1</sup> Hoi-Yin Hui,<sup>2</sup> Vito W. Scarola,<sup>2</sup> and Brian DeMarco<sup>1,\*</sup>

*<sup>1</sup>Department of Physics, University of Illinois at  
Urbana-Champaign, Urbana, Illinois 61801, USA*

*<sup>2</sup>Department of Physics, Virginia Tech, Blacksburg, Virginia 24061, USA*

(Dated: November 6, 2017)

---

\* bdemarco@illinois.edu

## I. EXPERIMENTAL SEQUENCE AND PARAMETERS

Ultracold gases composed of  $^{40}\text{K}$  atoms in the  $|F = 9/2, m_F = 9/2\rangle$  and  $|F = 9/2, m_F = 7/2\rangle$  states are cooled to temperatures below the Fermi temperature  $T_F$  in a crossed-beam 1064 nm optical dipole trap using standard techniques. After evaporative cooling, the optical trap depth is increased to the same value for all the data presented in this paper. The resulting dipole trap frequencies are  $(47.9 \pm 0.4)$  Hz,  $(98 \pm 1)$  Hz, and  $(114 \pm 2)$  Hz. A microwave-frequency swept magnetic field combined with a static magnetic field gradient are used to remove all atoms in one hyperfine state, thereby preparing a spin-polarized gas before we ramp on the three pairs of lattice beams in 100 ms. The Raman beams are derived from a cavity-stabilized diode laser (Vortex II TLB-6900) and are 80 GHz red-detuned from the  $D1$  transition. The frequency and power of each beam are controlled using an acousto-optic modulator.

A 13 G magnetic field is used to lift the degeneracy of Zeeman transitions between different  $m_F$  states. The field provides a 27kHz difference between the  $m_F = 9/2 \rightarrow 7/2$  and  $m_F = 7/2 \rightarrow 5/2$  transitions. No significant population of  $m_F = 5/2$  atoms has been observed in our measurements. The drift in the magnetic field is about 10 mG from day-to-day and 3 mG over the course of two-hour measurement run.

The magnetic field is reduced to 3 G for imaging. An additional magnetic field gradient is applied during time-of-flight to spatially separate the two spin components. A gaussian distribution is used to fit the images of each spin component and determine the corresponding atom number.

## II. THEORETICAL DESCRIPTION OF EFFECTIVE CSFT HAMILTONIAN

### A. Single-Particle Hamiltonian

We first review the Raman-transition Hamiltonian in the absence of interactions and a lattice. Consider a three-level atom in the presence of two red-detuned lasers, described by

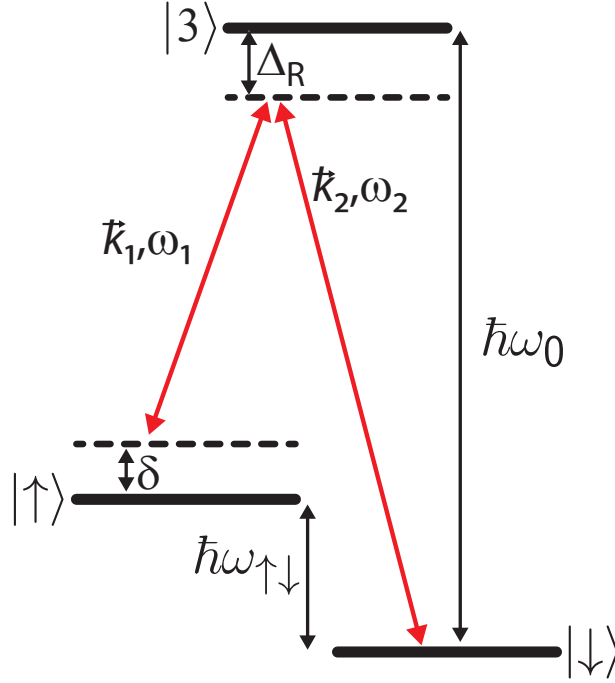

FIG. S1. Energy levels of a 3-level atoms with two lasers of frequencies  $\omega_1$  and  $\omega_2$ .

the level diagram shown in Fig. S1. The Hamiltonian is

$$H_{3\text{-lev}} = \begin{pmatrix} \omega_{\uparrow\downarrow} & 0 & \frac{\Omega_1^*}{2} (e^{-i(\vec{k}_1 \cdot \vec{R} - \omega_1 t)} + \text{c.c.}) \\ 0 & 0 & \frac{\Omega_2^*}{2} (e^{-i(\vec{k}_2 \cdot \vec{R} - \omega_2 t)} + \text{c.c.}) \\ \frac{\Omega_1}{2} (e^{i(\vec{k}_1 \cdot \vec{R} - \omega_1 t)} + \text{c.c.}) & \frac{\Omega_2}{2} (e^{i(\vec{k}_2 \cdot \vec{R} - \omega_2 t)} + \text{c.c.}) & \omega_0 \end{pmatrix}, \quad (1)$$

which is written with respect to the  $\{|\uparrow\rangle, |\downarrow\rangle, |3\rangle\}$  basis. Here,  $\vec{R}$  is the position of the atom, the laser frequencies satisfy  $\omega_1 = \omega_0 - \Delta_R - \delta - \omega_{\uparrow\downarrow}$  and  $\omega_2 = \omega_0 - \Delta_R$ , and  $\Omega_{1,2} = -e \cdot \langle 3 | \vec{E}_{1,2} \cdot \vec{r} | \uparrow, \downarrow \rangle$  are the dipole matrix elements for the atom-light (with electric field  $\vec{E}_i$ ) interaction. For the calculations in the main text and discussed in this document, we use a simplified model in which laser beam 1 only couples  $|\uparrow\rangle$  and  $|3\rangle$ , and laser beam 2 only couples  $|\downarrow\rangle$  and  $|3\rangle$ . In the experiment, the polarizations of the Raman beams are such that both ground states are coupled to the (multi-level) excited state by both beams.

We make the rotating-wave approximation and a unitary transformation  $H'_{3\text{-lev}} = e^{i \int^t V dt'} H_{3\text{-lev}} e^{-i \int^t V dt'} - V$ , with

$$V = \begin{pmatrix} \omega_{\uparrow\downarrow} + \delta & 0 & 0 \\ 0 & 0 & 0 \\ 0 & 0 & \omega_0 - \Delta_R \end{pmatrix}, \quad (2)$$

which is similar to a transformation to a rotating frame. Projecting  $H'_{3\text{-lev}}$  onto the subspace  $\{|\uparrow\rangle, |\downarrow\rangle\}$ , under the condition  $|\Omega_1| \approx |\Omega_2| \ll \Delta_R$ , yields

$$H_{2\text{-lev}} \approx \begin{pmatrix} \delta & \frac{\Omega}{2} e^{-i\vec{\delta}k \cdot \vec{R}} \\ \frac{\Omega^*}{2} e^{i\vec{\delta}k \cdot \vec{R}} & 0 \end{pmatrix}, \quad (3)$$

for an effective Hamiltonian, where  $\Omega = -\Omega_1^* \Omega_2 / 2\Delta_R$  and  $\vec{\delta}k = \vec{k}_1 - \vec{k}_2$ . This projection is equivalent to adiabatically eliminating the excited electronic state. These two levels act as the pseudo-spin basis used in the main part of the text.

## B. Lattice and Interaction Effects

In the presence of an optical lattice, we project the Hamiltonian onto the lowest Bloch band of the lattice. We denote the Wannier function centered at the site located at  $\vec{R}_i$  as  $\psi_i(\vec{r}) = \psi(\vec{r} - \vec{R}_i)$  and  $c_{i\sigma}^\dagger$  as the operator that creates a fermion with spin  $\sigma$  at that site. The full tight-binding Hamiltonian is

$$H_0 = -t \sum_{\langle ij \rangle \sigma} (c_{i\sigma}^\dagger c_{j\sigma} + \text{hc}) + \sum_{\langle ij \rangle} \left( \frac{\Omega}{2} e^{-i\vec{\delta}k \cdot \frac{\vec{R}_i + \vec{R}_j}{2}} \Psi_{ij} c_{i\uparrow}^\dagger c_{j\downarrow} + i \leftrightarrow j + \text{hc} \right) \\ + \sum_i \left( \frac{\Omega}{2} \Psi_0 e^{-i\vec{\delta}k \cdot \vec{R}_i} c_{i\uparrow}^\dagger c_{i\downarrow} + \frac{\Omega^*}{2} \Psi_0 e^{i\vec{\delta}k \cdot \vec{R}_i} c_{i\downarrow}^\dagger c_{i\uparrow} \right) + \frac{\delta}{2} \sum_i (n_{i\uparrow} - n_{i\downarrow}) + U \sum_i n_{i\uparrow} n_{i\downarrow}, \quad (4)$$

where  $n_{i\sigma} = c_{i\sigma}^\dagger c_{i\sigma}$ ,  $\Psi_{ij} = \int d\vec{r} \psi_i^* e^{i\vec{\delta}k \cdot (\vec{R}_i - \vec{R}_j)} \psi_j$  is a Debye-Waller factor,  $\Psi_0 = \Psi_{00}$ , and  $U$  is the strength of on-site interaction. The first term is the ordinary spin-conserving tunneling term. The second term is a spin-flip tunneling term akin to spin-orbit coupling in the lattice. The third term is an on-site spin-flip term, which can be understood as an effective Zeeman term in the  $x, y$  directions. The fourth term is an effective Zeeman energy. For the experimental parameters explored in this work, we find  $\Psi_{ij} \approx \delta_{ij}$ . The second term can therefore be safely ignored.

## C. Effective Hamiltonian for $\delta \approx U$

To derive an effective Hamiltonian for CSFT, we work in the limit  $U, \delta \gg t, \Omega$  and treat the first three terms of  $H_0$  as perturbations. We consider the case  $\delta \approx U$  and choose to require exact energy conservation between final states and the initial spin-polarized state. Off-resonant processes that can, for example, lead to sites occupied by a single spin-down

atom are ignored. We therefore project our Hamiltonian onto such states where all sites obey  $\langle n_{i\downarrow}(1 - n_{i\uparrow}) \rangle = 0$ . Let  $\mathcal{P}$  be the projector onto this space. Second-order perturbation theory then gives

$$\begin{aligned}
H_{\text{eff}} = & \mathcal{P} \left[ -t \sum_{\langle ij \rangle \sigma} (c_{i\sigma}^\dagger c_{j\sigma} + \text{hc}) - \frac{t\Psi_0}{2} \left( \frac{1}{U} + \frac{1}{\delta} \right) \sum_{\langle ij \rangle} \left( \frac{\Omega^*}{2} (e^{i\delta\vec{k}\cdot\vec{R}_i} - e^{i\delta\vec{k}\cdot\vec{R}_j}) c_{i\downarrow}^\dagger c_{j\uparrow} + i \leftrightarrow j + \text{hc} \right) \right. \\
& + \left( \frac{\delta}{2} + \frac{|\Omega|^2 \Psi_0^2}{4\delta} \right) \sum_i (n_{i\uparrow} - n_{i\downarrow}) + U \sum_i n_{i\uparrow} n_{i\downarrow} \\
& + \sum_{\langle ij \rangle} \left( \frac{\Omega}{2} e^{-i\delta\vec{k}\cdot\frac{\vec{R}_i + \vec{R}_j}{2}} \Psi_{ij} c_{i\uparrow}^\dagger c_{j\downarrow} + i \leftrightarrow j + \text{hc} \right) + \frac{2t^2}{U} \sum_{\langle ij \rangle} (c_{i\uparrow}^\dagger c_{i\downarrow}^\dagger c_{j\downarrow} c_{j\uparrow} + \text{hc}) \\
& + \frac{2t^2}{U} \sum_{\langle ij \rangle} (n_{i\uparrow} n_{i\downarrow} (1 - n_{j\uparrow}) (1 - n_{j\downarrow}) + i \leftrightarrow j) + \frac{t^2}{U} \sum_{\langle ij \rangle, \langle ij' \rangle, j \neq j'} n_{i\uparrow} c_{i\downarrow}^\dagger c_{j'\downarrow} c_{j\downarrow}^\dagger c_{i\downarrow} \\
& \left. + \frac{t^2}{U} \sum_{\langle ij \rangle, \langle ij' \rangle, j \neq j'} (1 - n_{i\downarrow}) c_{j\uparrow}^\dagger c_{i\uparrow}^\dagger c_{i\downarrow}^\dagger c_{j'\uparrow} - \frac{t^2}{U} \sum_{\langle ij \rangle, \langle ij' \rangle, j \neq j'} (c_{j\uparrow}^\dagger c_{j'\downarrow}^\dagger c_{i\uparrow} c_{i\downarrow} + \text{hc}) \right] \mathcal{P}.
\end{aligned} \tag{5}$$

Noting that  $\Psi_{ij} \approx 0$  for  $i \neq j$  and further ignoring higher-order interactions, this can be written as

$$\begin{aligned}
H_{\text{eff}} = & \mathcal{P} \left[ -t \sum_{\langle ij \rangle \sigma} (c_{i\sigma}^\dagger c_{j\sigma} + \text{hc}) + \sum_{\langle ij \rangle} (K_{ij} c_{j\uparrow}^\dagger c_{i\downarrow} + K_{ji} c_{i\uparrow}^\dagger c_{j\downarrow} + \text{hc}) \right. \\
& \left. + \frac{\delta^*}{2} \sum_i (n_{i\uparrow} - n_{i\downarrow}) + U \sum_i n_{i\uparrow} n_{i\downarrow} \right] \mathcal{P} + \mathcal{O}\left(\frac{t^2}{U}\right),
\end{aligned} \tag{6}$$

where

$$K_{ij} = -t\Omega\Psi_0 \frac{e^{-i\delta\vec{k}\cdot\vec{R}_i} - e^{-i\delta\vec{k}\cdot\vec{R}_j}}{4} \left( \frac{1}{U} + \frac{1}{\delta} \right) \tag{7}$$

$$\delta^* = \delta + \frac{|\Omega\Psi_0|^2}{2\delta}. \tag{8}$$

$H_{\text{eff}}$  governs the dynamics of fully polarized initial states discussed in the main text. The first term moves (but does not create) doublons and holes (e.g.,  $|\uparrow\downarrow, \downarrow\rangle \rightarrow |\downarrow, \uparrow\downarrow\rangle$ ). The second term is a spin-flip tunneling, which due to the projectors  $\mathcal{P}$  is effective only if no sites with spin-down are created. We can therefore rewrite the second term by explicitly inserting the projectors:  $K_{ij} n_{i\uparrow} (1 - n_{j\downarrow}) c_{j\uparrow}^\dagger c_{i\downarrow} + i \leftrightarrow j + \text{hc}$ . This term can create doublon-hole pairs out of the fully polarized initial state and dominates the dynamics to leading order.

#### D. Estimation of $U$ Using the Resonance Near $\delta = U$

The value of the Hubbard  $U$  is estimated experimentally via CSFT by finding the resonant  $\delta$  at which doublon creation is most effective. As discussed in the main text, this procedure appears to undervalue  $U$  compared with the tight-binding prediction from independent measurements of the lattice potential depth. To understand how higher order terms in  $H_{\text{eff}}$  may explain this discrepancy, we consider a two-site system with the three states  $|\uparrow, \uparrow\rangle, |\uparrow\downarrow, 0\rangle, |0, \uparrow\downarrow\rangle$  and solve for the value of  $\delta$  at which the doublon creation rate is maximized. Writing  $H_{\text{eff}}$  in this basis,

$$\begin{aligned} H_{\text{eff}}^{(2)} &= \begin{pmatrix} \delta + \frac{\Psi_0^2 |\Omega|^2}{2\delta} & K_{12} & -K_{21} \\ K_{12}^* & U + \frac{2t^2}{U} & \frac{2t^2}{U} \\ -K_{21}^* & \frac{2t^2}{U} & U + \frac{2t^2}{U} \end{pmatrix} \\ &= \mathcal{U}^\dagger \begin{pmatrix} \delta + \frac{\Psi_0^2 |\Omega|^2}{2\delta} & \sqrt{2}K_{12} & 0 \\ \sqrt{2}K_{12}^* & U + \frac{4t^2}{U} & 0 \\ 0 & 0 & U \end{pmatrix} \mathcal{U} \end{aligned} \quad (9)$$

where  $\mathcal{U}$  transforms the basis to  $\left\{ |\uparrow, \uparrow\rangle, \frac{|\uparrow\downarrow, 0\rangle + |0, \uparrow\downarrow\rangle}{\sqrt{2}}, \frac{|\uparrow\downarrow, 0\rangle - |0, \uparrow\downarrow\rangle}{\sqrt{2}} \right\}$ , and the equality  $K_{ij} = -K_{ji}$  has been used. The first two states have the same energy (and hence doublon creation is most effective) when:

$$\begin{aligned} \delta + \frac{\Psi_0^2 |\Omega|^2}{2\delta} &= U + \frac{4t^2}{U} \\ \delta &\approx U + \frac{4t^2 - |\Omega|^2 \Psi_0^2 / 2}{U} + \frac{2t^2 |\Omega|^2 \Psi_0^2}{U^3} \end{aligned} \quad (10)$$

Here we see that the resonant condition for maximal doublon creation is not exactly at  $\delta = U$ , but instead shows higher-order corrections. These corrections contribute to the deviation between the measured and predicted  $U$  discussed in the main text.

#### E. Validating the CSFT Effective Model

The effective model  $H_{\text{eff}}$  is a perturbative result, in comparison to the full tight-binding Hamiltonian  $H_0$ . To test the validity of the dynamics predicted by  $H_{\text{eff}}$ , we compare the time evolution of the double occupancy in both models.

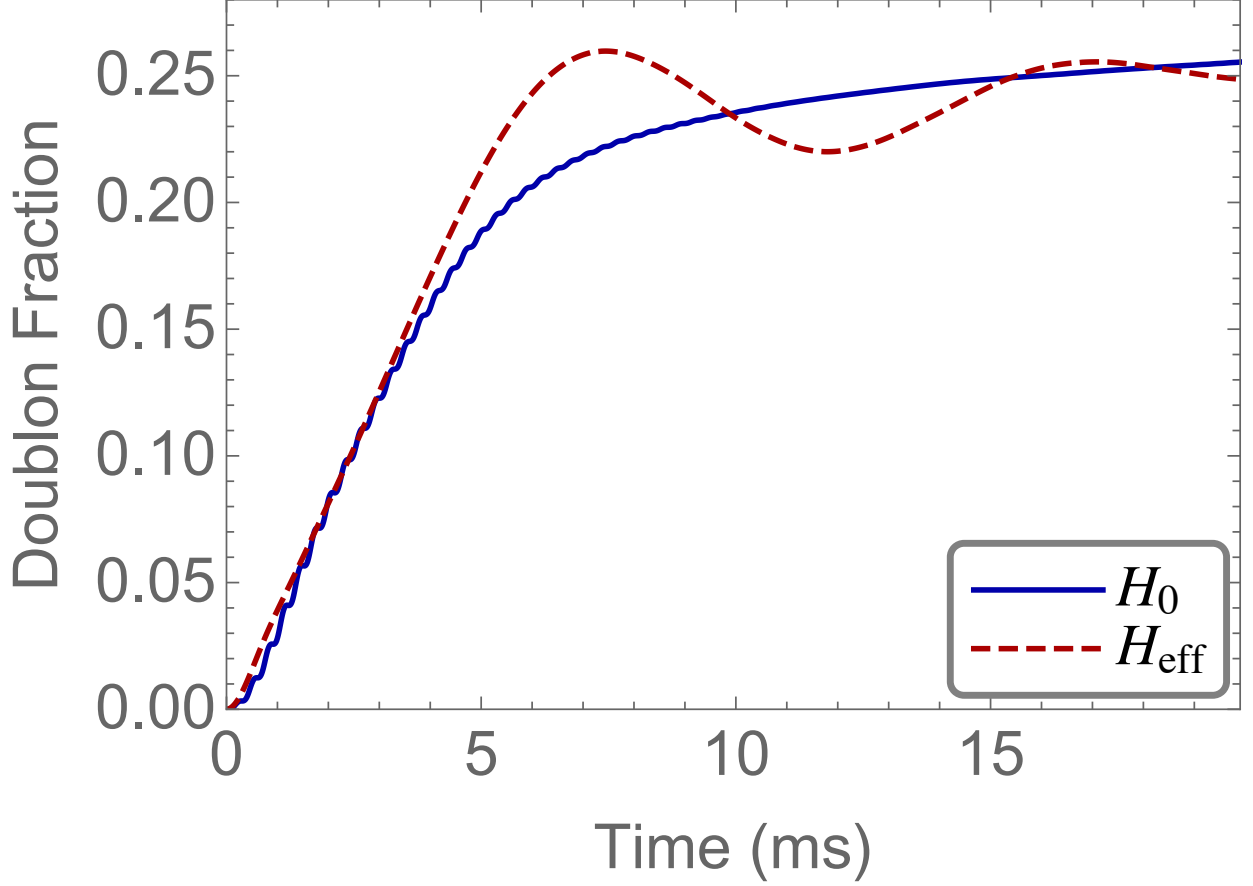

FIG. S2. The evolution of doublon fraction  $\langle n_{i\uparrow}n_{i\downarrow} \rangle / \langle n_{i\uparrow} + n_{i\downarrow} \rangle$  from a numerical simulation with constant  $\Omega$ . The solid lines shows the simulation with the full Hamiltonian  $H_0$ , while the dashed line shows that with the effective Hamiltonian  $H_{\text{eff}}$  derived from second-order perturbation theory. The states are initialized with one spin-up fermion on every site, and the parameters are determined by experiment:  $t/h = 0.25\text{kHz}$ ,  $U/h = 3.22\text{kHz}$ ,  $\Omega = 0.1U$  and  $\vec{\delta}\vec{k} \cdot \vec{d} = \pi/2\sqrt{3}$ .

The dynamics of  $H_0$  cannot be solved exactly in large systems with dimension higher than one. We therefore consider doublon dynamics in one-dimension. We initialize a one-dimensional infinite system with one spin-up fermion in each state, and evolve it with infinite time-evolving block decimation (iTEBD) [1]. The evolution of doublon fraction, defined as  $D = \langle n_{i\uparrow}n_{i\downarrow} \rangle / \langle n_{i\uparrow} + n_{i\downarrow} \rangle$ , is plotted in Fig. S2(a). The simulations performed with  $H_0$  and  $H_{\text{eff}}$  are both presented.

Here we see that the effective model captures the qualitative features of the full Hamiltonian. The doublon creation rate at short times is essentially the same for both models. Furthermore, the long-time steady-state reveals approximately the same doublon fraction.

In both models the timescale of equilibration is roughly set by  $\hbar/|K_{\langle ij \rangle}| = 14\text{ms}$ . We therefore see that the effective CSFT model  $H_{\text{eff}}$  captures the essential features of the full tight-binding model  $H_0$ .

## F. CSFT Timescale: Theory–Experiment Comparison

We measure the Rabi rate of the carrier  $\Psi_0 |\Omega| = 2\pi \times 650 \text{ Hz}$  using resonant Rabi oscillations. The carrier frequency  $\omega_{\uparrow\downarrow}$  is determined using a fit of the spin transition probability vs. Raman detuning  $\Delta\omega$  for a 0.7 ms pulse, which is too short to drive CSFT.

Measuring the slower rate for CSFT requires a longer timescale. We eliminate the background contribution from the broad carrier feature using the same procedure as for Fig. 4 in the main text. After locating the carrier frequency  $\omega_{\uparrow\downarrow}$ , we perform two measurements with the same Raman pulse time at  $\Delta\omega = \omega_{\uparrow\downarrow} + U/\hbar$ , but with different initial spin polarization. The difference between these two measurements  $f_{\uparrow} - f_{\downarrow}$  reflects only the CSFT process. Fig. S3 shows the measured CSFT signal for different Raman pulse times at  $s = 8 E_R$  lattice depth.

The measured CSFT timescale is approximately a factor of five larger than that of the numerical simulations shown in Fig. S2, which use the experimentally determined carrier Rabi rate. The uncertainty in  $t$  and  $U$  (which determine  $K_{ij}$  and the CSFT timescale) from measurements of the lattice potential depth are too small to support this difference.

A potential source of this discrepancy is phase-noise between the Raman laser beams, which translates into fluctuations in the complex phase of  $|\Omega|$  in  $H_{\text{eff}}$ . Phase noise with a non-uniform frequency spectrum is required to explain this inconsistency, since the predicted CSFT time dependence shown in Fig. S2 is constrained by all the experimental parameters, including the independent measurement of  $|\Omega|$  using the carrier transition. In order to differentially affect the carrier and CSFT transitions, the phase-noise spectral density must be frequency dependent.

To explore this, we carry out iTEBD numerical simulations with a time-dependent  $\Omega e^{i\phi(t)}$ . The result, plotted as the solid line in Fig. S3, shows better agreement with the experimental result. We reserve a detailed discussion of the noise and comparison with experiment to future work [2].

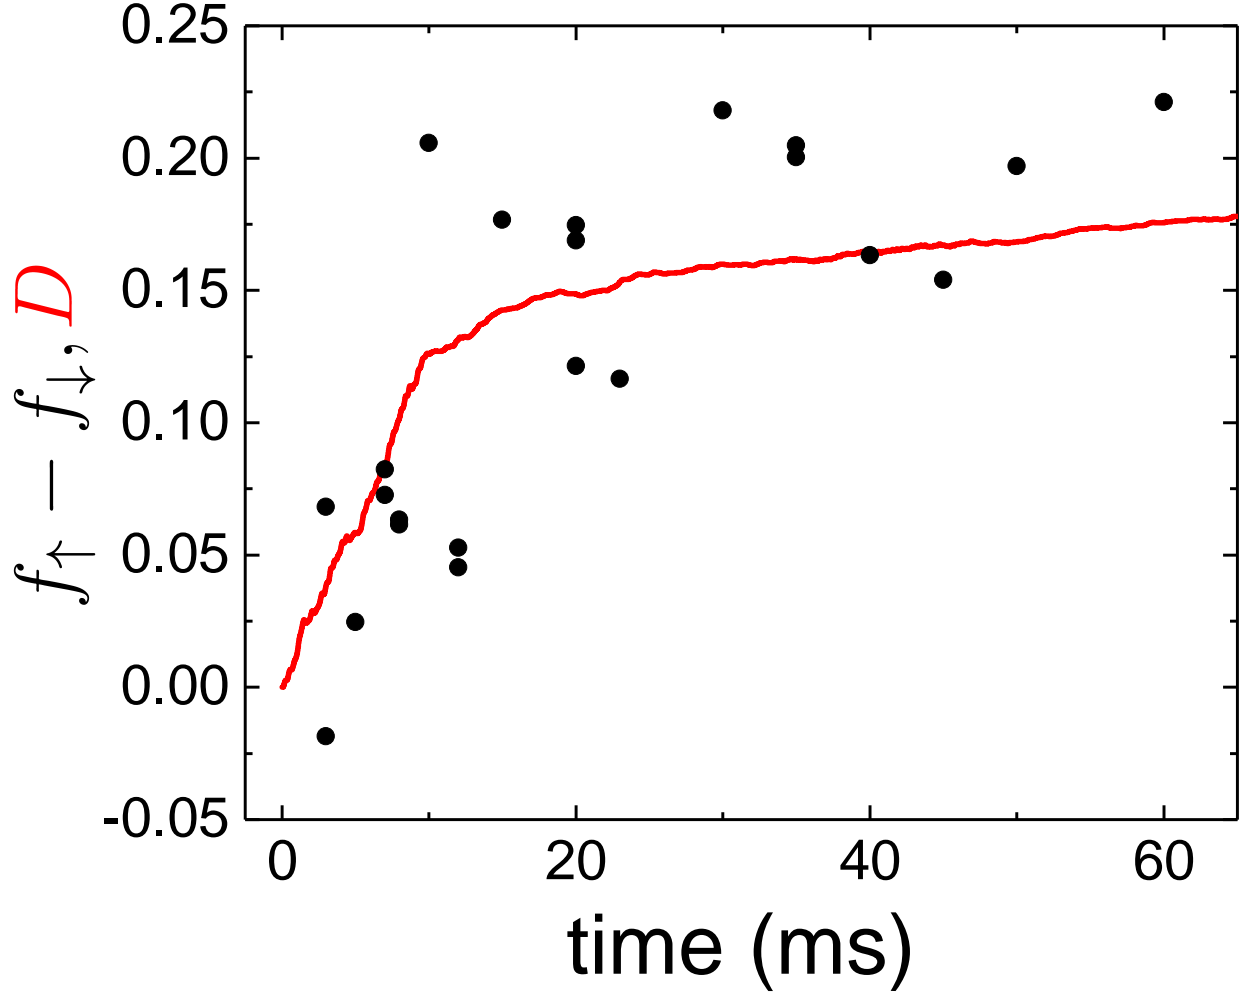

FIG. S3. CSFT signal for varied Raman pulse time. The Raman detuning for these measurements is fixed to the  $+U$  CSFT sideband. The measurements are shown using black circles, and a theoretical simulation is displayed as a red line. The simulation is performed with  $\Omega$  in  $H_0$  replaced with  $\Omega e^{i\phi(t)}$ , where  $\langle\langle\phi(t)^2\rangle\rangle=8$ , and the characteristic timescale of the fluctuations in  $\phi(t)$  is 2 ms. The dynamics has been averaged (indicated by the notation  $\langle\langle\rangle\rangle$ ) over five realizations of  $\phi(t)$ . For these parameters, the carrier Rabi oscillations are not strongly perturbed.

### III. RAMAN PHASE GRADIENT

As discussed in the main text, the spatially dependent Raman phase that arises because the Raman beams intersect at an angle plays a key role in enabling CSFT. We use a two-site, two-atom toy model to explain how the Raman phase disrupts destructive interference between multiple tunneling pathways that is induced by antisymmetrization of the

wavefunction.

Considering a two-site, two-fermion system, there are 6 possible configurations, which we label according to the site and spin occupancy in each well:  $|\uparrow, \uparrow\rangle_W$ ,  $|\downarrow, \downarrow\rangle_W$ ,  $|\downarrow, 0\rangle_W$ ,  $|0, \uparrow\downarrow\rangle_W$ ,  $|\uparrow, \downarrow\rangle_W$ , and  $|\downarrow, \uparrow\rangle_W$ . In this well-specific basis,  $|\downarrow, \uparrow\rangle_W$  means that a  $|\downarrow\rangle$  atom is in the left well (located at position  $\vec{R}_1$ ) and an  $|\uparrow\rangle$  atom is in the right well (located at position  $\vec{R}_2$ ), for example.

Using a Slater determinant to explicitly write down properly symmetrized (un-normalized) two-atom wavefunctions, we have:

$$|\uparrow, \uparrow\rangle_W = (|LR\rangle - |RL\rangle) |\uparrow\uparrow\rangle \quad (11)$$

$$|\downarrow, \downarrow\rangle_W = (|LR\rangle - |RL\rangle) |\downarrow\downarrow\rangle \quad (12)$$

$$|\downarrow\uparrow, 0\rangle_W = |LL\rangle (|\uparrow\downarrow\rangle - |\downarrow\uparrow\rangle) \quad (13)$$

$$|0, \downarrow\uparrow\rangle_W = |RR\rangle (|\uparrow\downarrow\rangle - |\downarrow\uparrow\rangle) \quad (14)$$

$$|\uparrow, \downarrow\rangle_W = (|LR\rangle - |RL\rangle)(|\uparrow\downarrow\rangle + |\downarrow\uparrow\rangle) + (|LR\rangle + |RL\rangle)(|\uparrow\downarrow\rangle - |\downarrow\uparrow\rangle) \quad (15)$$

$$|\downarrow, \uparrow\rangle_W = (|LR\rangle - |RL\rangle)(|\uparrow\downarrow\rangle + |\downarrow\uparrow\rangle) - (|LR\rangle + |RL\rangle)(|\uparrow\downarrow\rangle - |\downarrow\uparrow\rangle), \quad (16)$$

where the spatial part of the wavefunction is written in the basis of  $|L\rangle$  and  $|R\rangle$ , which are single-particle states on either the left or the right well, and the spin component is denoted as  $|\uparrow\rangle$  and  $|\downarrow\rangle$ . For example, in this basis,  $|LR\rangle |\uparrow\downarrow\rangle$  means that atom 1 is in the left well in the  $|\uparrow\rangle$  state, and atom 2 is in the right well in the  $|\downarrow\rangle$  state. The key point for this discussion is that the  $|\uparrow, \downarrow\rangle_W$  and  $|\downarrow, \uparrow\rangle_W$  states consist of spin singlet and triplet components. Furthermore, the relative sign between the spin and triplet components is opposite for these two states.

We focus on resonant CSFT with  $\Delta\omega = U/\hbar$ . An initially spin-polarized state  $|\uparrow, \uparrow\rangle_W$  (as in the experiment) can transition to a virtual state  $|\uparrow, \downarrow\rangle_W$  or  $|\downarrow, \uparrow\rangle_W$  via a Raman transition (see Fig. S4). The amplitude for this process is suppressed by a factor of  $1/U$  because of the energy mismatch. The phase of the virtual state depends on which atom undergoes a spin-flip, since  $\vec{\delta}k \neq 0$ . Therefore, the Raman phase enters as either  $e^{i\vec{\delta}k \cdot \vec{R}_1}$  or  $e^{i\vec{\delta}k \cdot \vec{R}_2}$ , where  $\vec{R}_1$  and  $\vec{R}_2$  differ by a lattice spacing  $\vec{d}$ . After the virtual state is formed, tunneling completes the CSFT process, and a doublon is formed. Via tunneling, the sign difference between equations 15 and 16 is converted into an overall sign difference between the wavefunctions for each doublon-formation pathway. This  $\pi$  relative phase between the wavefunctions can be computed from the tunneling matrix elements  $\langle \uparrow\downarrow, 0 |_W t(c_i^\dagger c_{i+1} + \text{h.c.}) | \uparrow, \downarrow \rangle_W$

and  $\langle \uparrow\downarrow, 0 |_W t(c_i^\dagger c_{i+1} + \text{h.c.}) |\downarrow, \uparrow\rangle_W$ .

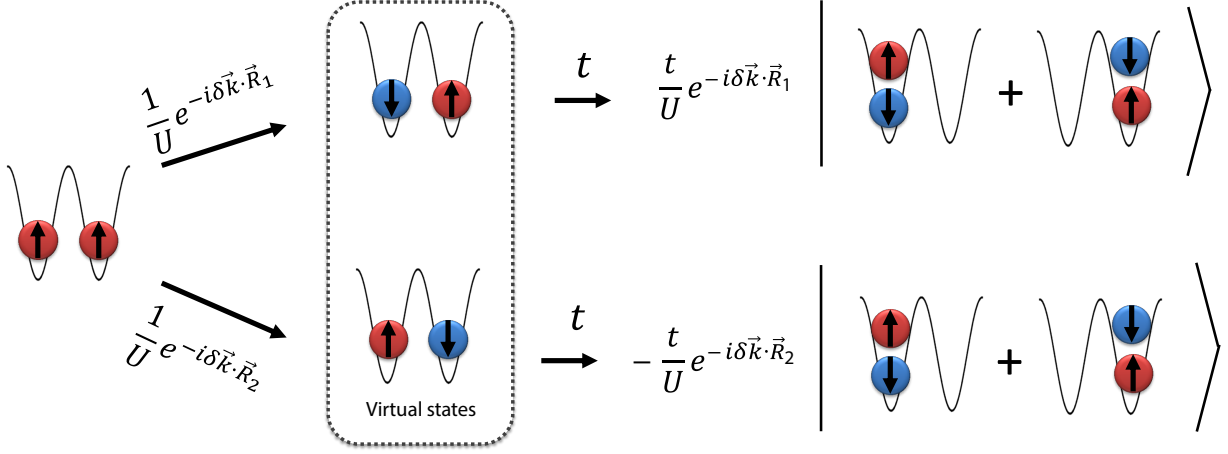

FIG. S4. A schematic diagram showing CSFT for a two-site two-fermion system. CSFT happens as a two-step process via a virtual state. Two possible channels between the initial state  $|\uparrow, \uparrow\rangle_W$  and the final state  $|\uparrow\downarrow, 0\rangle_W + |0, \uparrow\downarrow\rangle_W$  happen simultaneously but with amplitudes carrying opposite signs. The probability to observe a doublon-hole pair is affected by interference between these channels.

The transition between the between the initial state  $|\uparrow, \uparrow\rangle_W$  and the final doublon-hole state happens via these two possible channels simultaneously. The final state is a superposition of these two pathways, with a wavefunction proportional to  $(e^{-i\delta\vec{k}\cdot\vec{R}_1} - e^{-i\delta\vec{k}\cdot\vec{R}_2})(|\uparrow\downarrow, 0\rangle + |0, \uparrow\downarrow\rangle)$ . The probability to observe a doublon-hole state is thus proportional to  $[1 - \cos(\delta\vec{k}\cdot\vec{d})]$ . Without the Raman phase gradient (i.e.,  $\delta\vec{k} = 0$  or  $\delta\vec{k}\cdot\vec{d} = 0$ ), destructive interference prevents tunneling, and doublons will not be formed. Ultimately, this interference arises from the different signs between the triplet and singlet components in equations 15 and 16—it is absent for bosons, for instance.

#### IV. SIMULATION OF CSFT SENSITIVITY TO VACANCIES

We developed a simple numerical simulation (shown in Fig. 4 in the main text) to determine the sensitivity of CSFT to vacancies in the lattice. We compute a density distribution in the non-interacting limit, and determine the probability that neighboring sites are occupied as atoms are randomly removed. The density distribution after turning on the lattice is generated according to  $n(r_x, r_y, r_z) = \int \frac{d^3\vec{q}}{h^3} \frac{1}{e^{\beta[V(r_x, r_y, r_z) + \epsilon(\vec{q}) - \mu]} + 1}$ , where  $V(r_x, r_y, r_z)$  is the

total harmonic potential imposed by optical trap and lattice beams,  $\mu$  is the chemical potential,  $\beta = 1/k_B\tilde{T}$ ,  $\epsilon(\vec{q}) = 2t(3 - \cos \pi q_x/q_B - \cos \pi q_y/q_B - \cos \pi q_z/q_B)$  is the lattice dispersion,  $q_B = \hbar\pi/d$ , and  $\tilde{T}$  the effective temperature in the lattice. Both  $\mu$  and  $\tilde{T}$  are solved by matching the entropy and number of atoms  $N$  to the corresponding values in the dipole trap. Non-interacting thermodynamics (including the tight-binding lattice dispersion and confining potential) are solved to relate the entropy to  $N$  and  $\tilde{T}$ . Each site in the simulated lattice is computed as occupied by a single atom or empty based on comparing a random number in the interval  $[0, 1]$  to  $n(r_x, r_y, r_z)$ .

Atoms are randomly removed from the simulated density profile according to a probability  $\delta N$ , which corresponds to the average fraction of atoms discarded. The fraction  $N_p$  of atoms in adjacent occupied sites remaining after this removal procedure is counted. As shown in an inset to Fig. S5, atoms are only counted once if they participate in any nearest-neighbor pair. Results from this simulation for the fraction of atoms  $N_p$  are shown in Fig. S5 for  $N = 61000$  and entropy per particle  $S/N = 2.89k_B$  in the lattice. This curve is plotted in Fig. 4 in the main text.

We observe loss of atoms from heating caused by the Raman beams. To account for this effect,  $\delta N$  in our simulation includes loss induced by the Raman beams. For the measurements in Fig. 4 in the main text, the initial conditions before the controlled removal procedure are  $N = 80900 \pm 3940$ ,  $T/T_F = 0.29 \pm 0.04$ ;  $N = 54800 \pm 12500$ ,  $T/T_F = 0.34 \pm 0.04$ ; and  $N = 47200 \pm 2810$ ,  $T/T_F = 0.38 \pm 0.08$  from high to low  $\delta N$ . After removal and loss induced by the Raman beams, the atom number is  $59200 \pm 2660$ ,  $23700 \pm 1830$ , and  $10900 \pm 5180$ , from high to low  $\delta N$ .

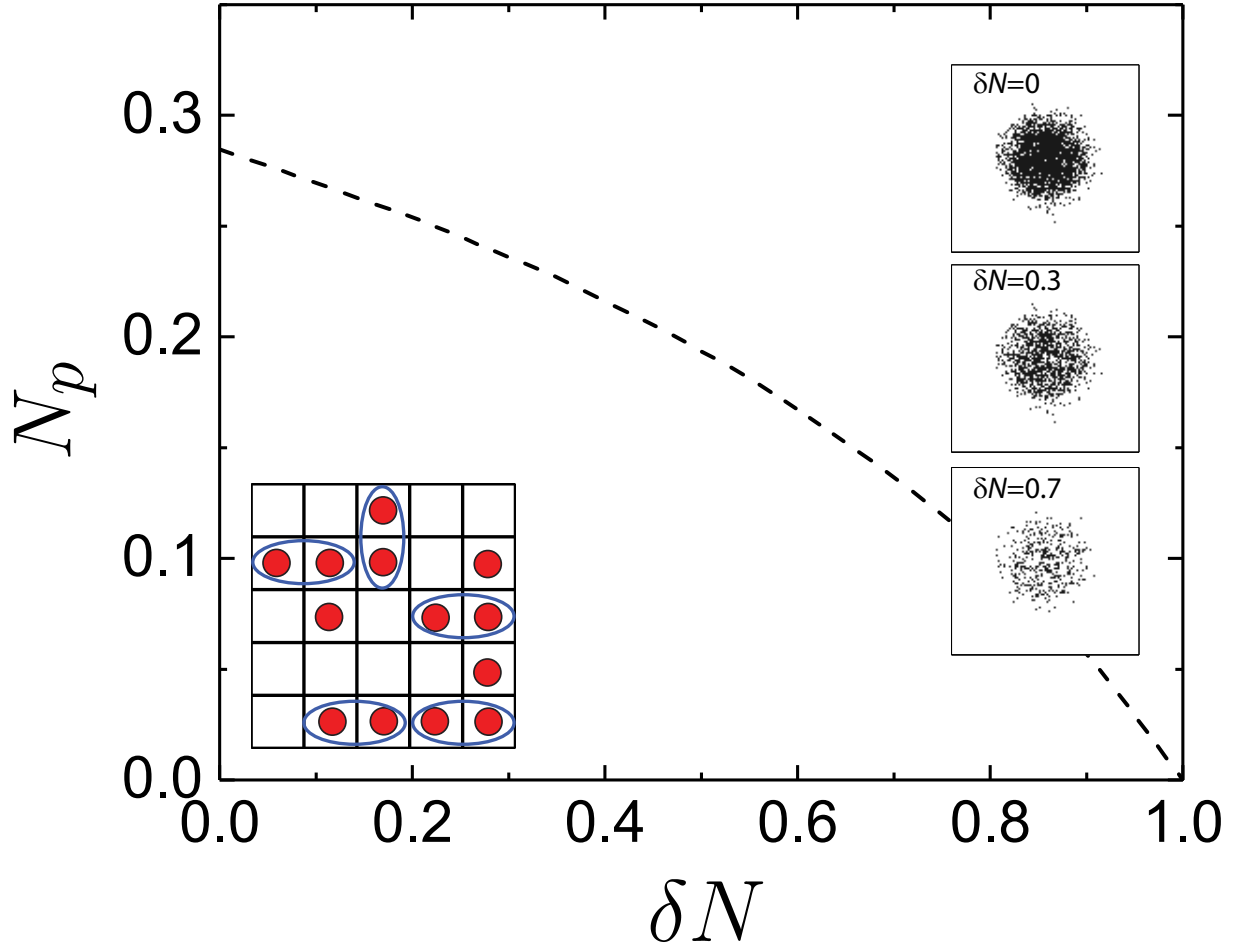

FIG. S5. The fraction of atoms with nearest neighbors at various removal fractions  $\delta N$  for  $N = 61000$  and  $S/N = 2.89 k_B$ , which corresponds to  $k_B \tilde{T} = 9.7t$  and chemical potential  $\mu = 6.4t$  in the lattice. The insets at the right show sample occupation profiles (with one black dot per atom) through a central slice of the gas. The inset at bottom left schematically illustrates the procedure for counting pairs.

- 
- [1] G. Vidal, Phys. Rev. Lett. **98**, 070201 (2007).
- [2] H.-Y. Hui, W. Xu, W. Morong, B. DeMarco, and V. Scarola, Unpublished.
